# Supplementary material for: SketchAgent: Language-Driven Sequential Sketch Generation
Source: arXiv:2411.17673 source file (2024-11-26)

butterfly

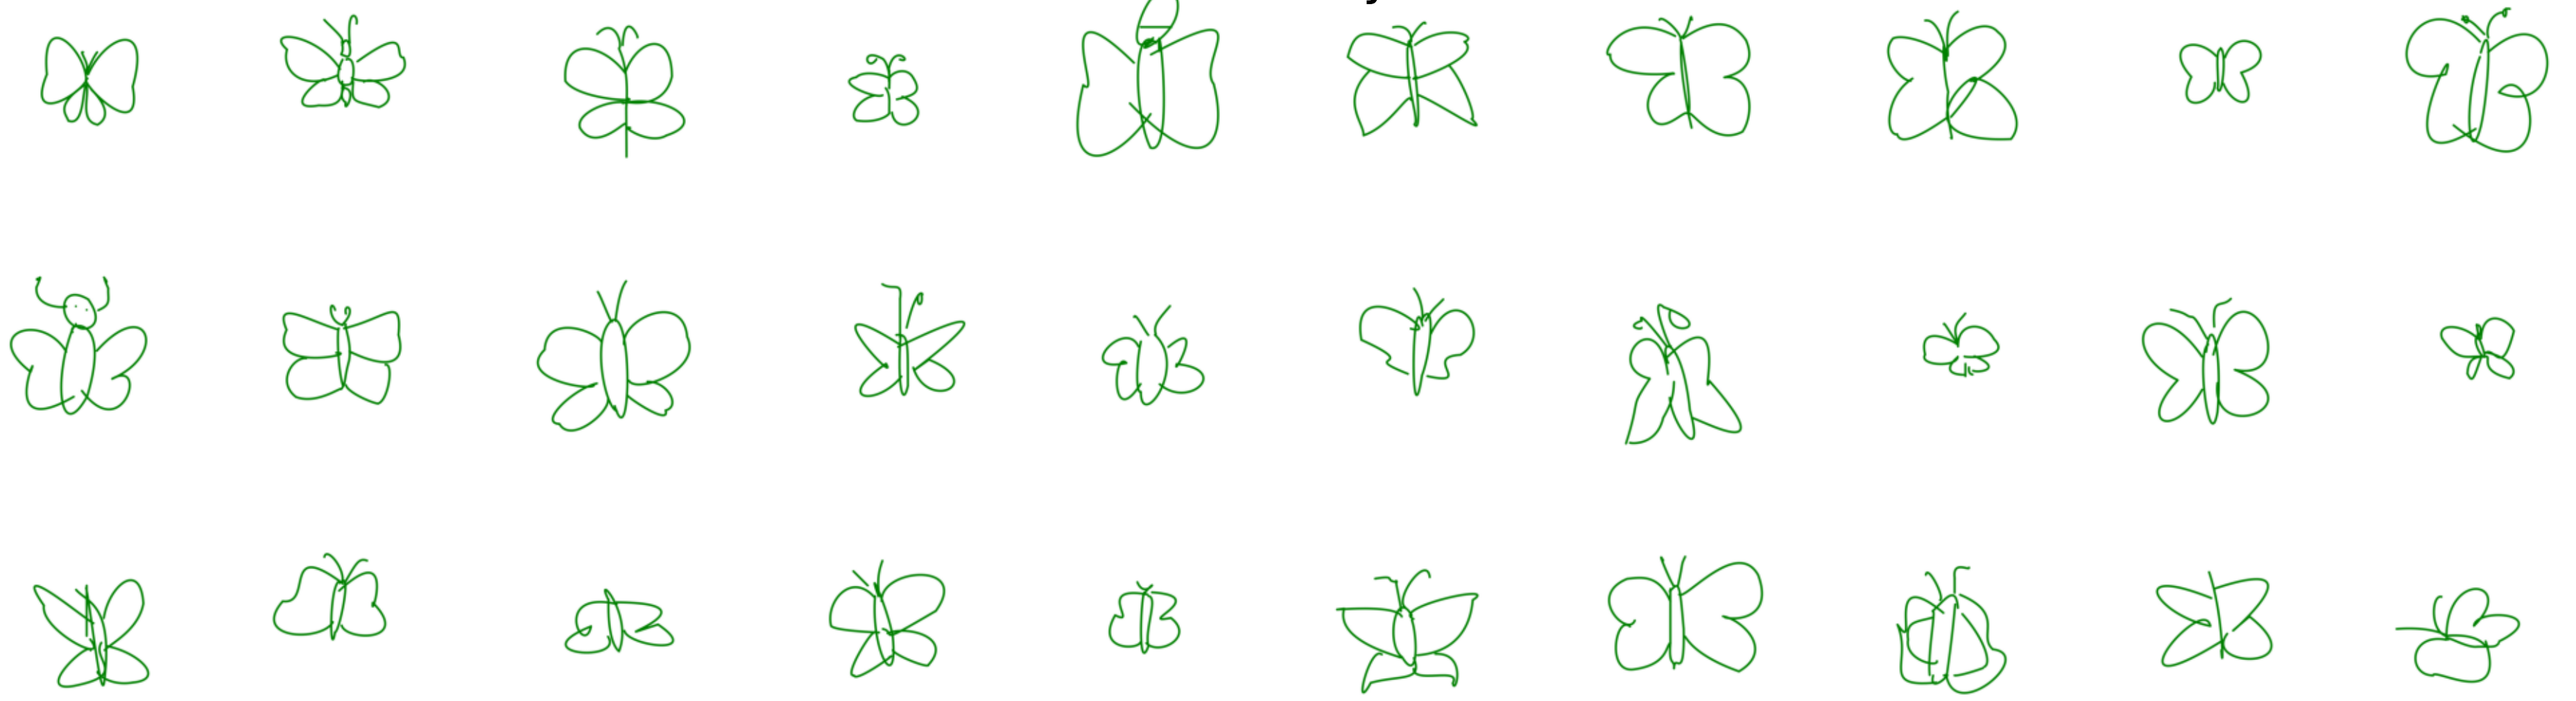

fish

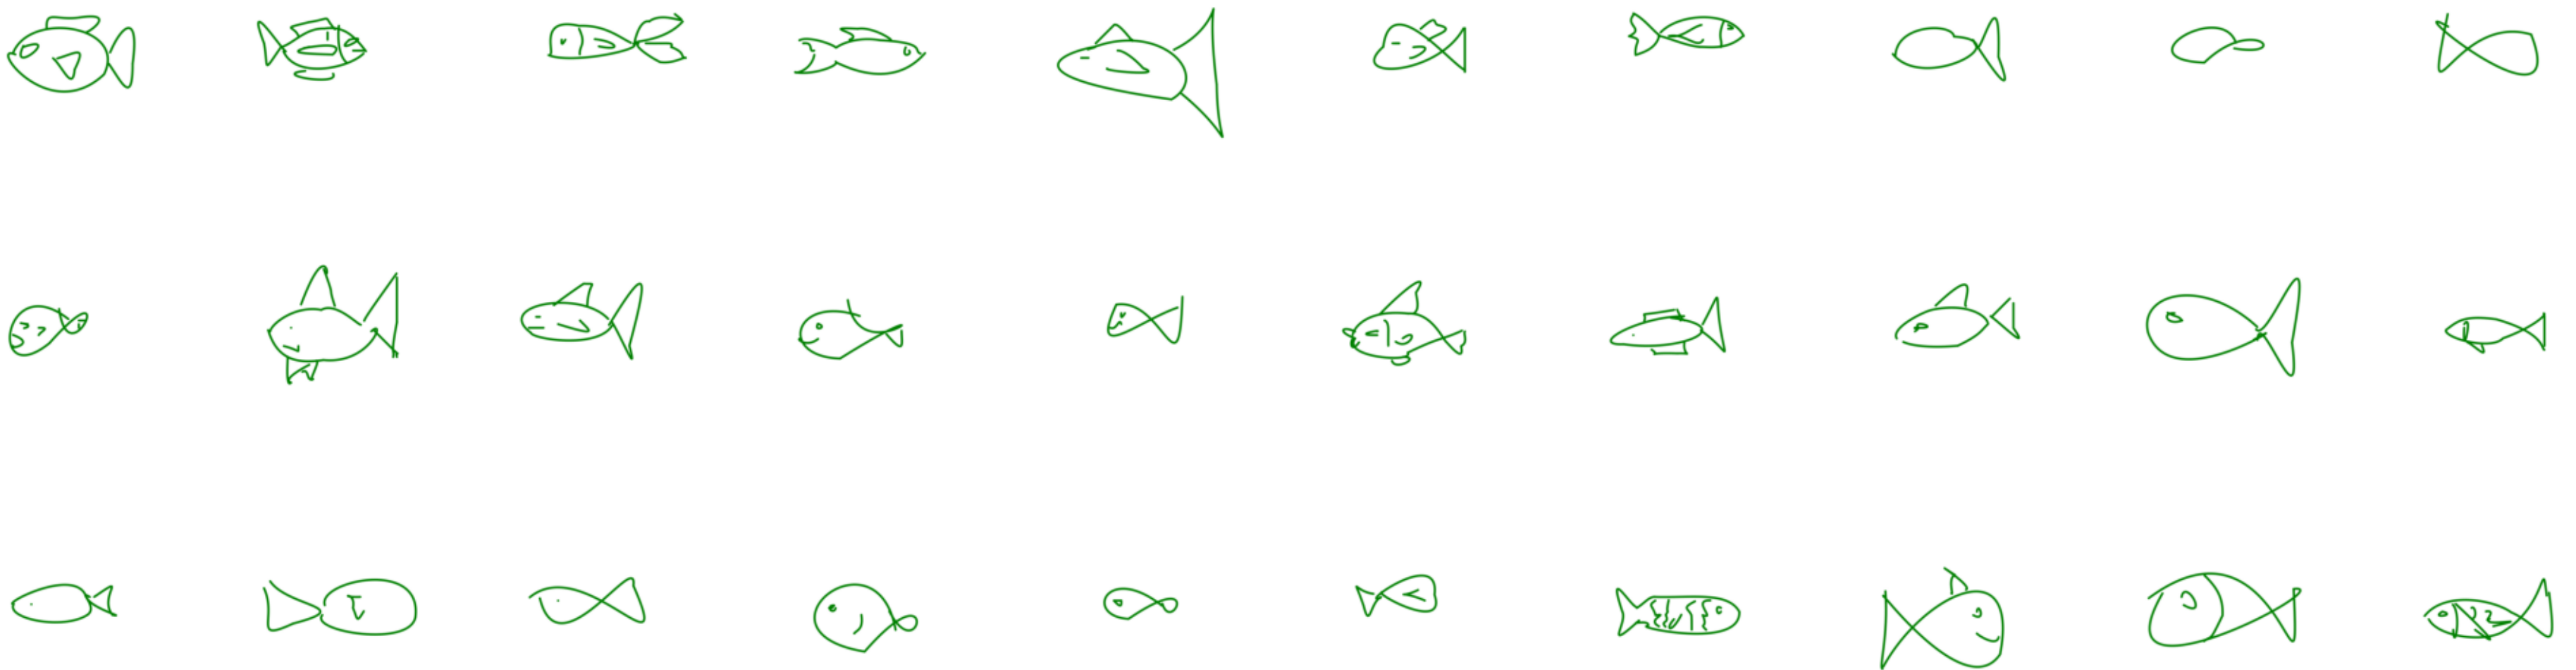

rabbit

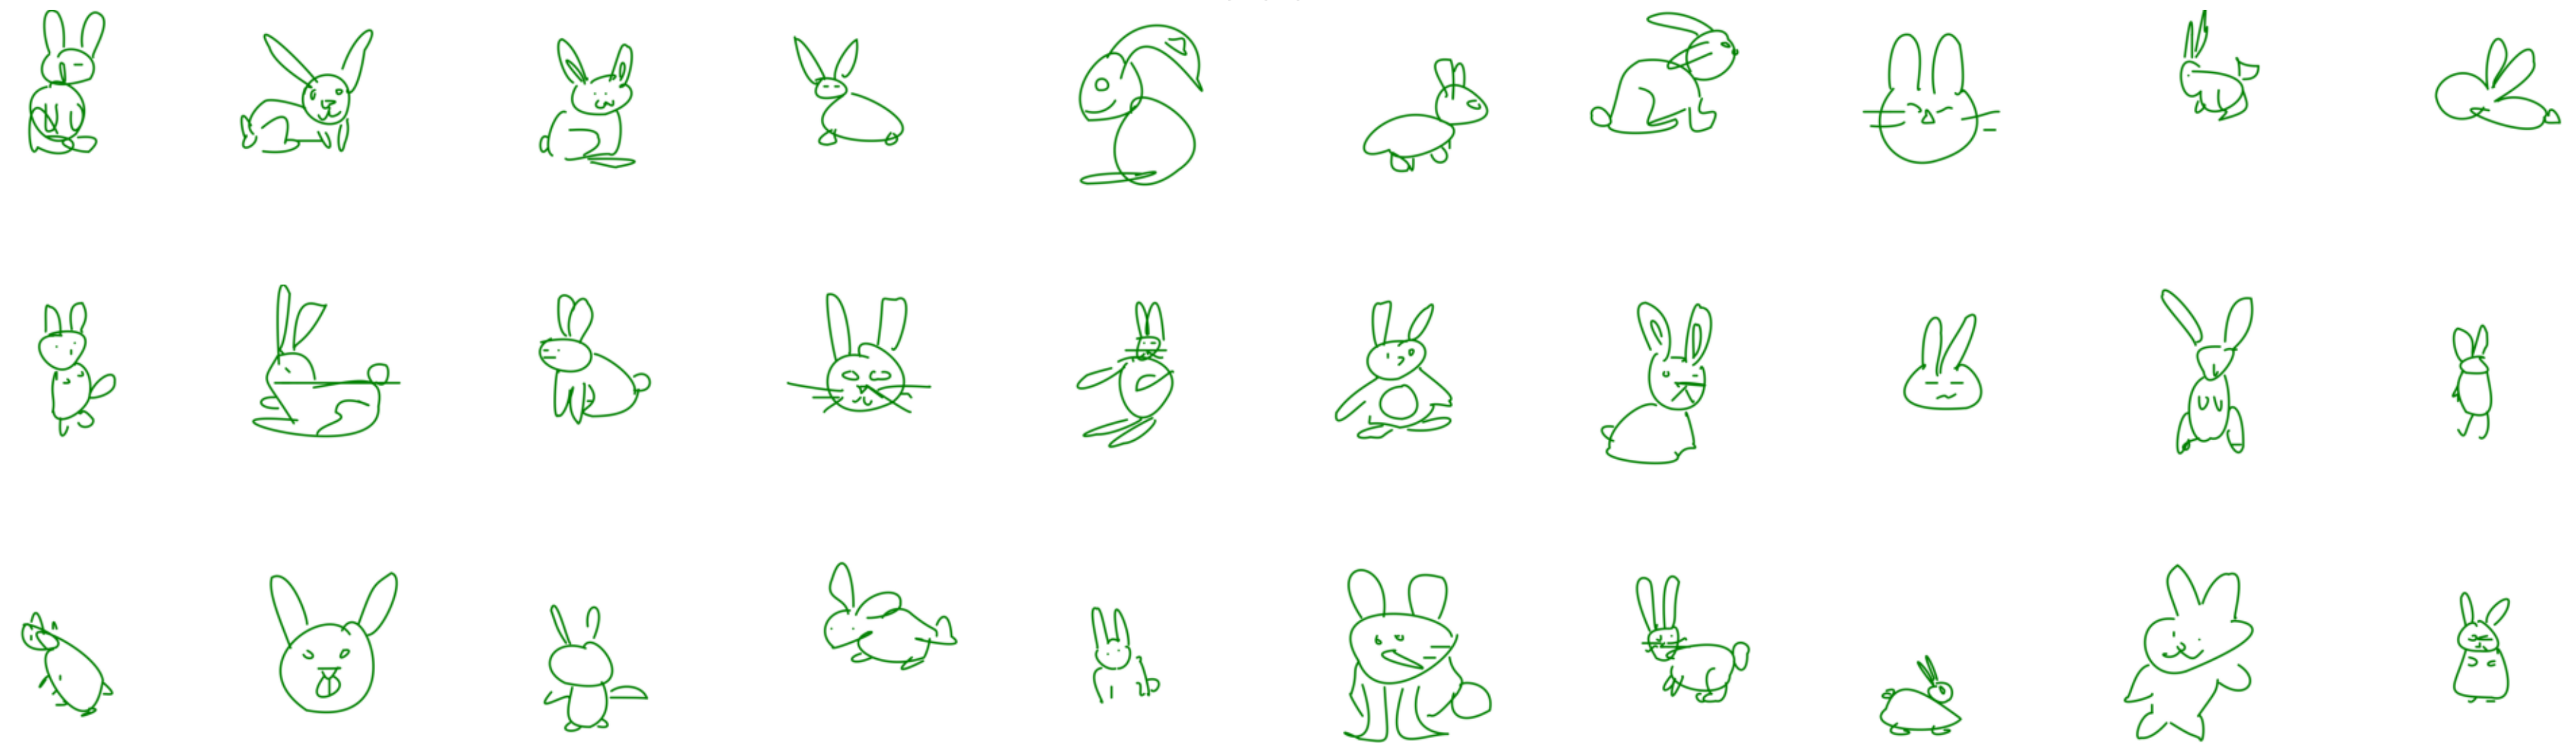

duck

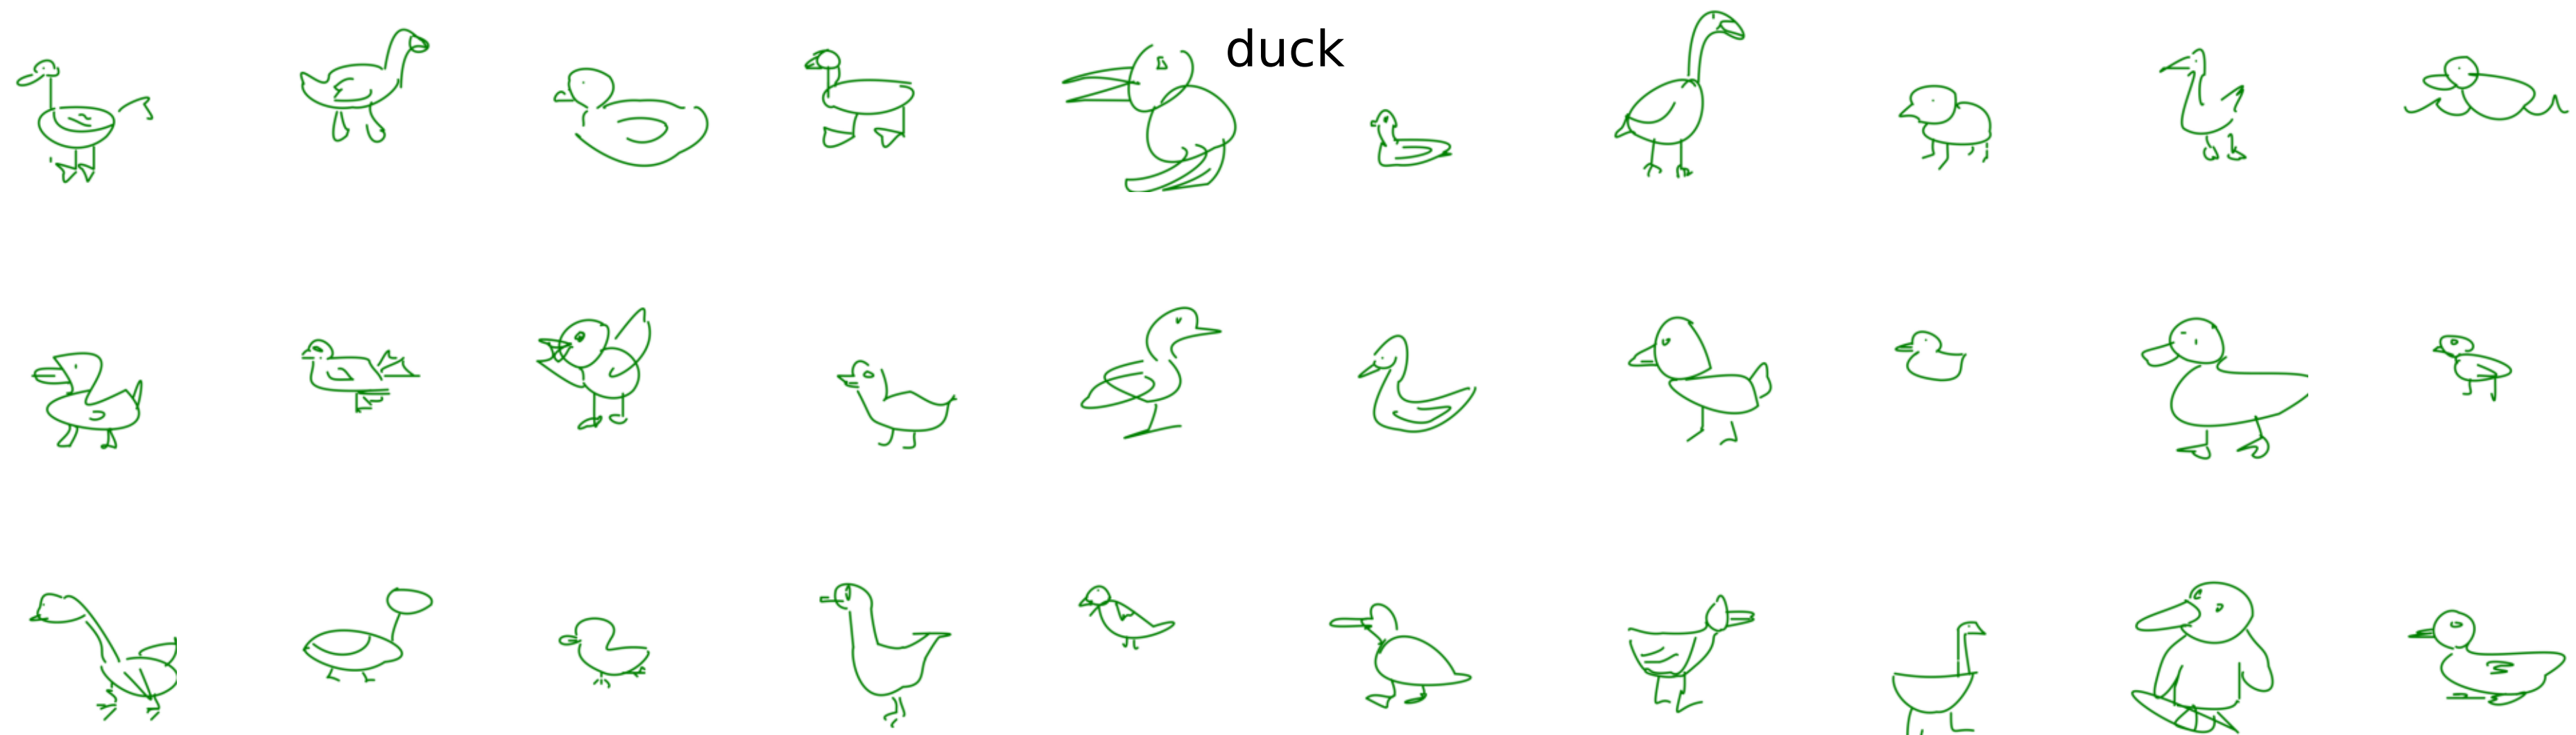

sailboat

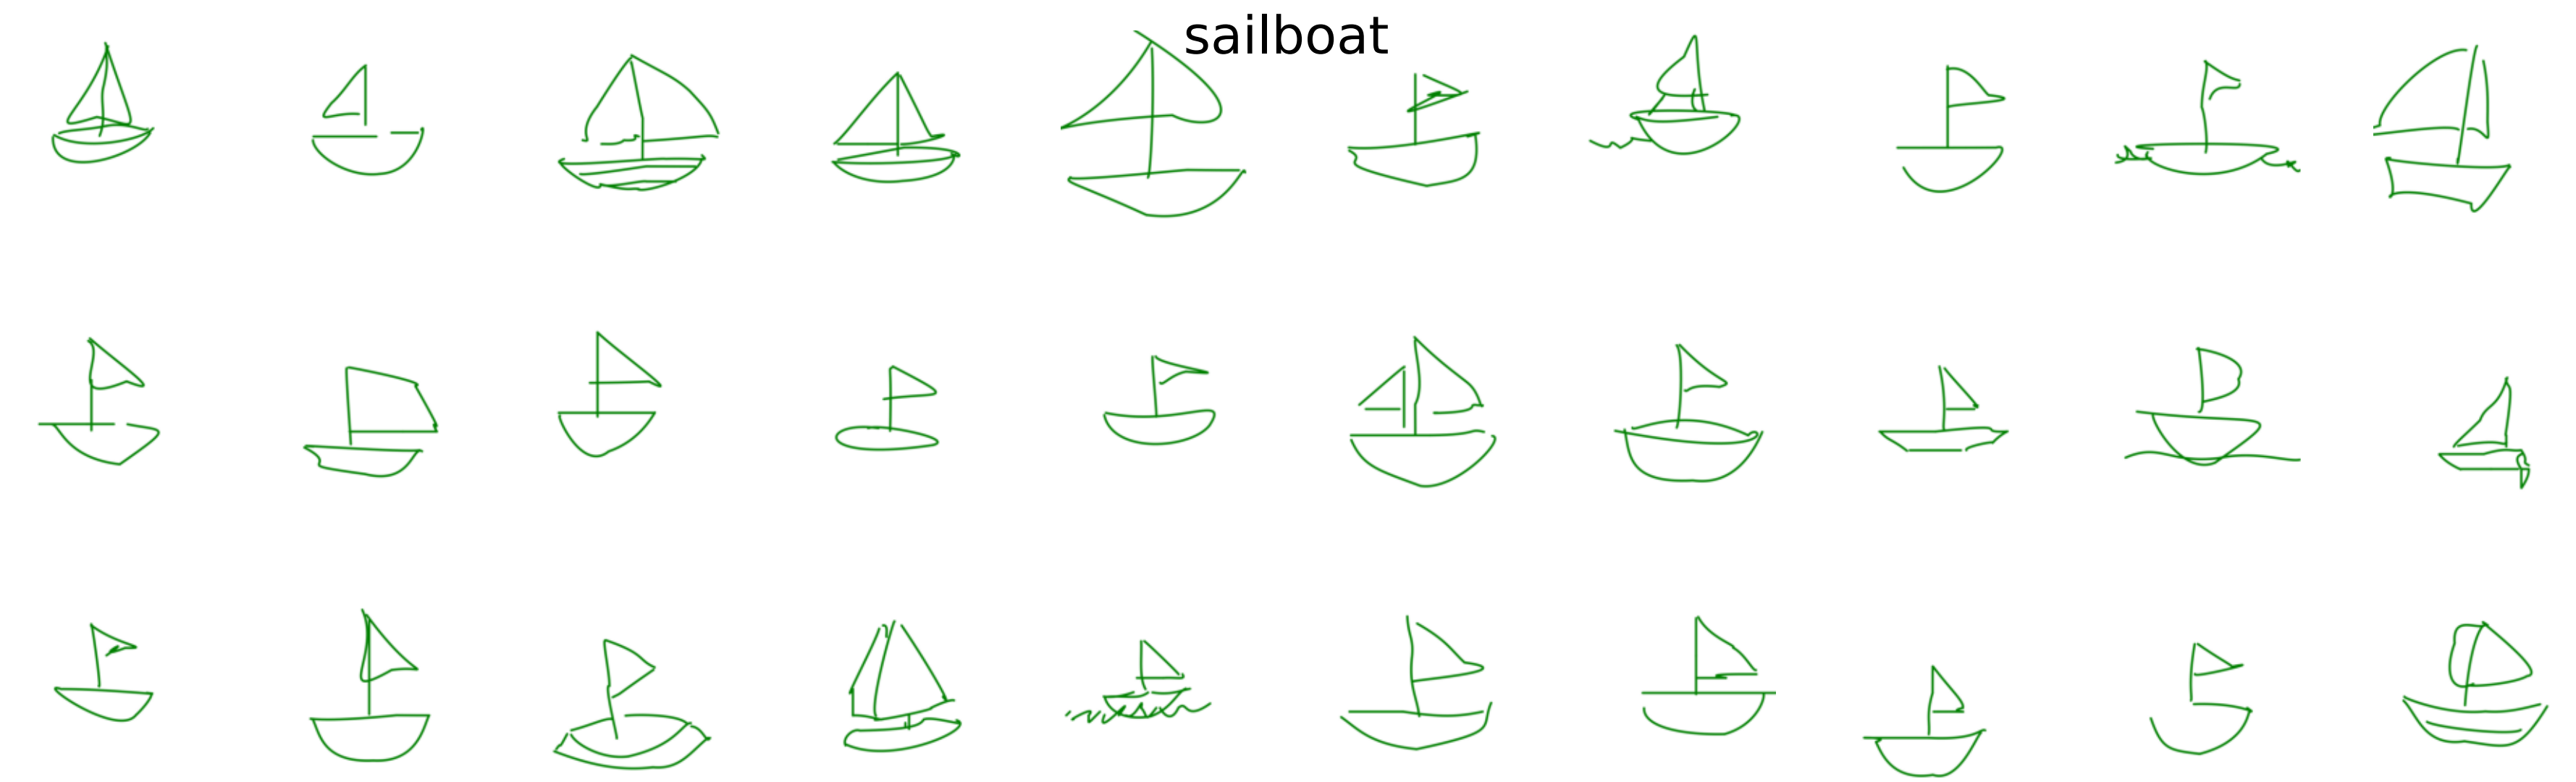

coffee mug

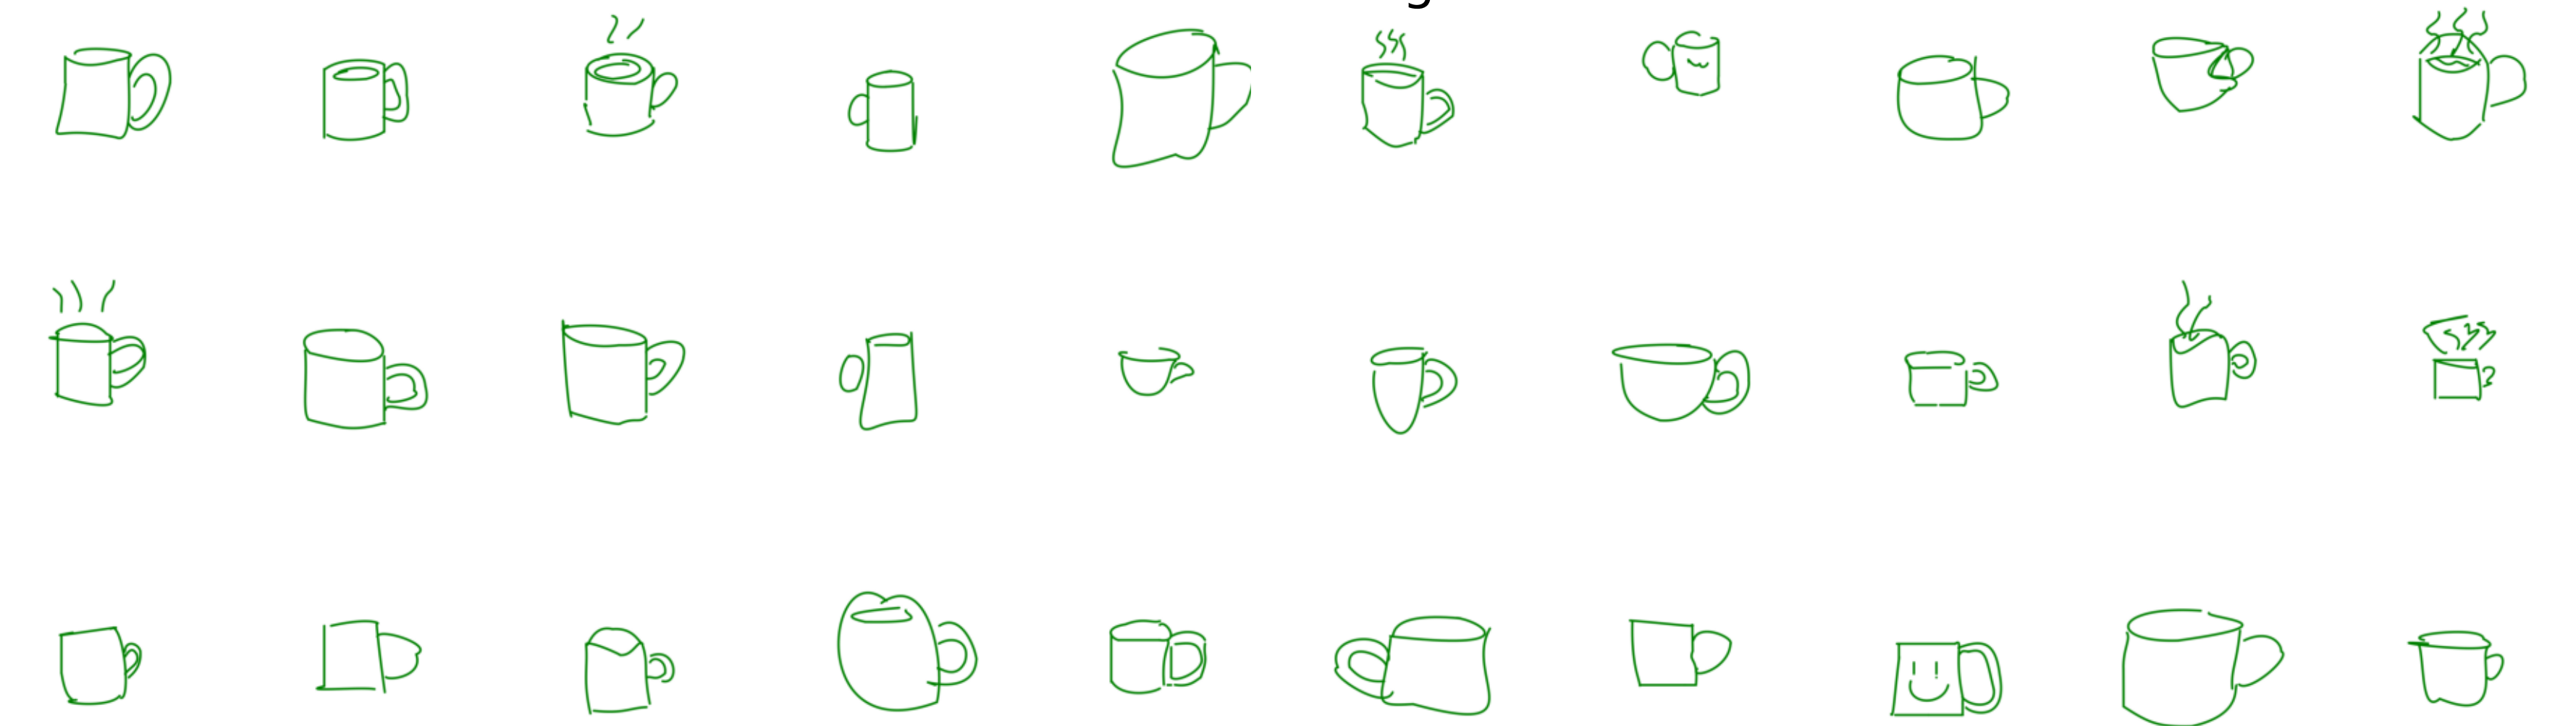

glasses

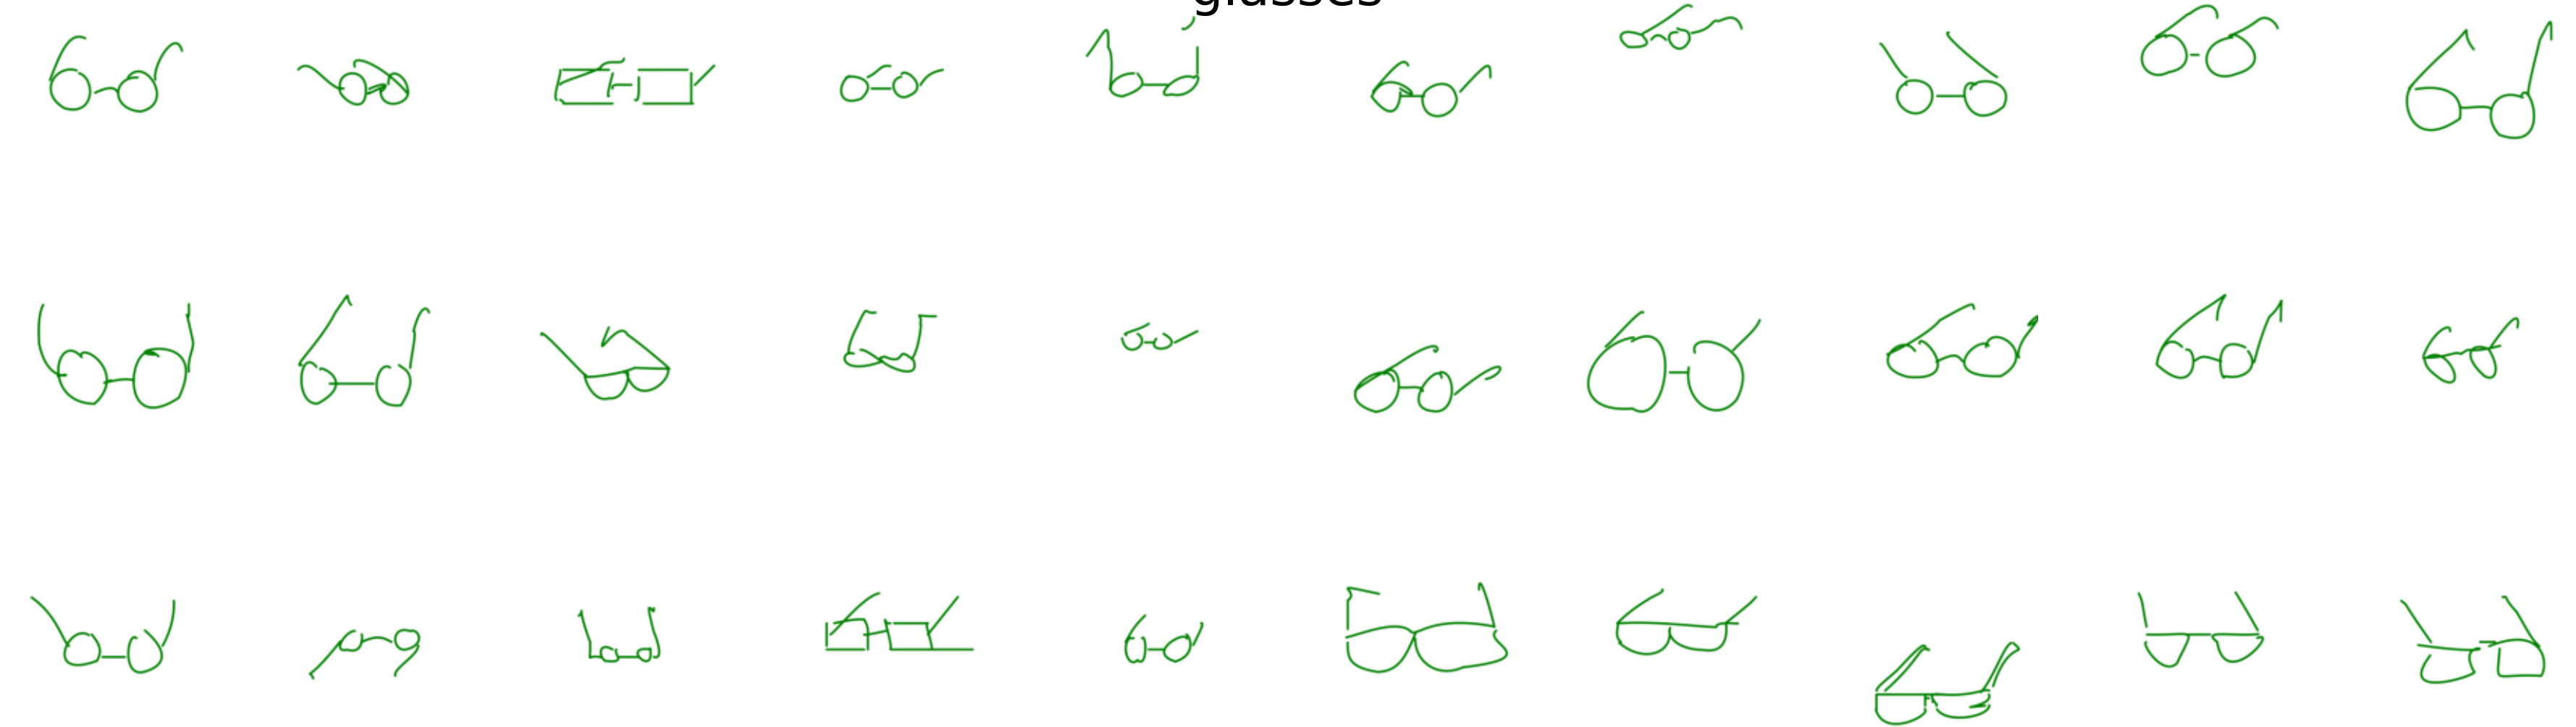

car

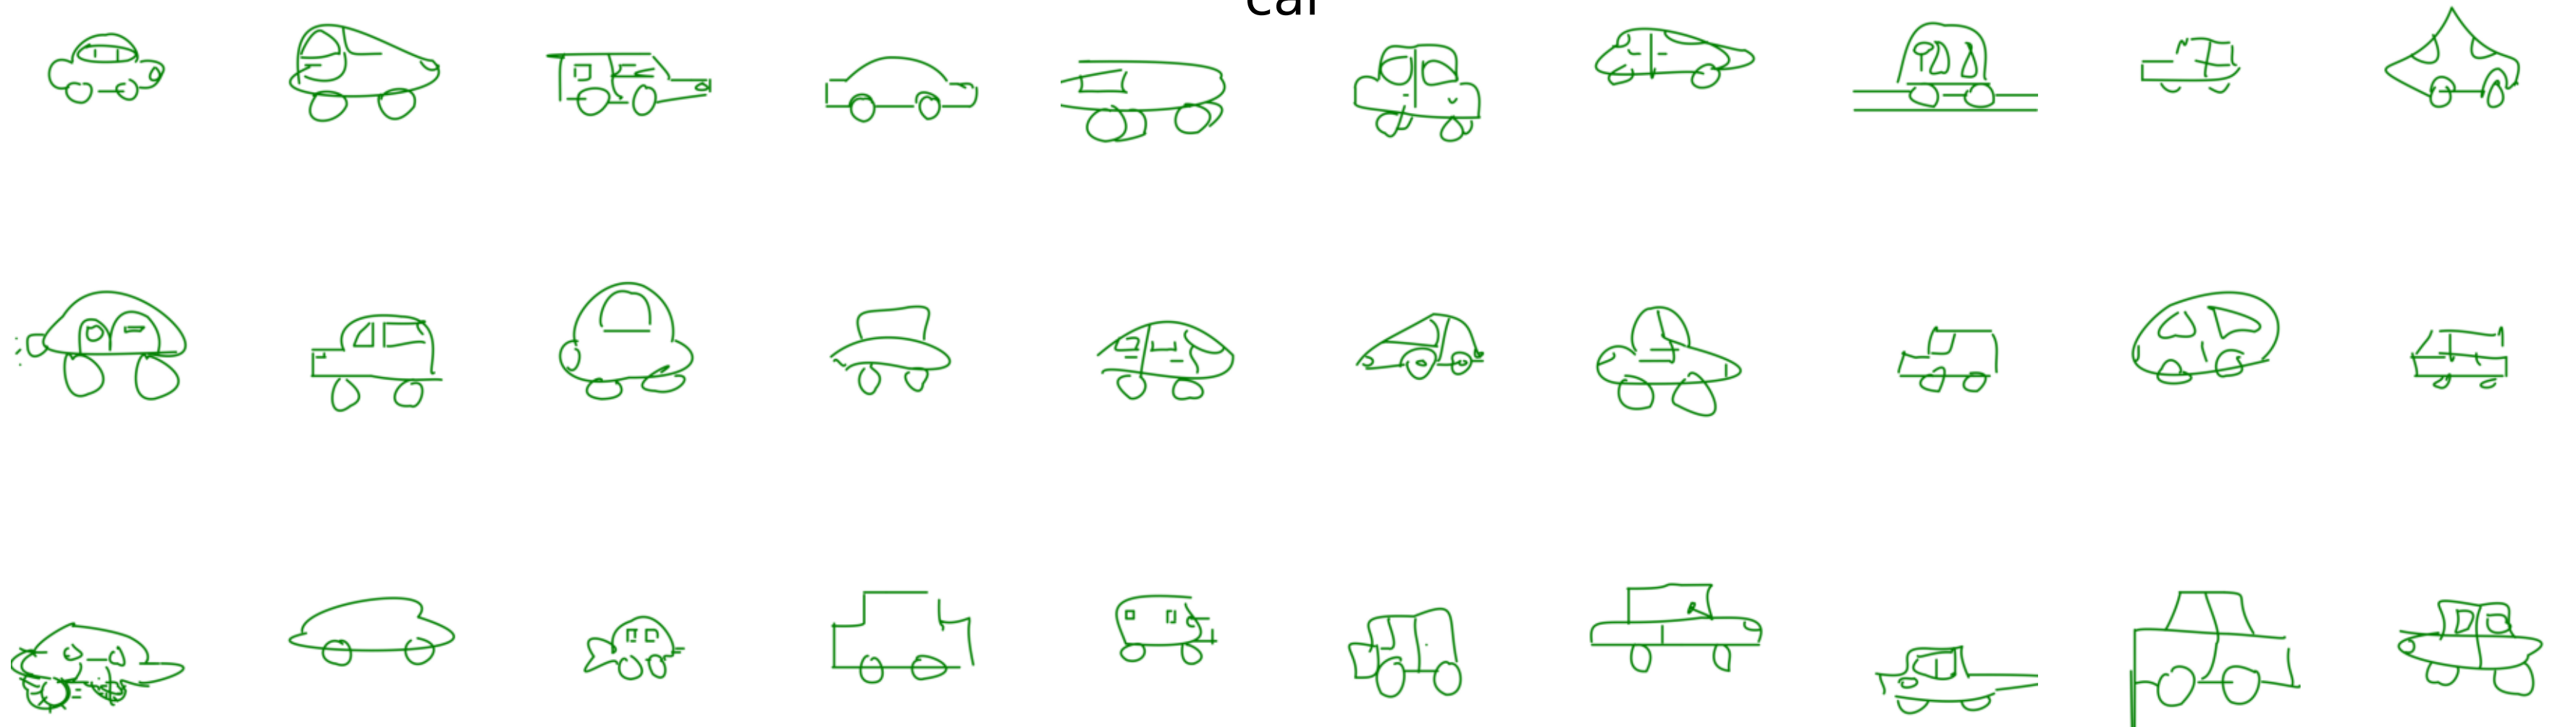

Supplement: Supplementary file 1 [file solo_user_all_2.pdf]
